# Supplementary material for: OT J002656.6+284933 (CSS101212:002657+284933): An SU UMa-Type Dwarf Nova with Longest Superhump Period
Source: arXiv:1703.00650 source file (2017-03-22)
Supplement: Supplementary file 1 [file si.pdf]

**E-table 1.** Log of Observations

| Start* | End* | Mean mag | error | $N^{\dagger}$ | Observer‡ | Filter |
|---|---|---|---|---|---|---|
| 2457689.2311 | 2457689.4061 | 15.247 | 0.006 | 236 | Kai | C |
| 2457689.4511 | 2457689.5670 | 15.094 | 0.007 | 163 | Trt | C |
| 2457691.2807 | 2457691.5412 | 15.156 | 0.004 | 336 | Trt | C |
| 2457691.3118 | 2457691.4995 | 15.330 | 0.005 | 246 | Kai | C |
| 2457692.1928 | 2457692.5217 | 15.226 | 0.004 | 438 | Trt | C |
| 2457692.2136 | 2457692.5009 | 15.480 | 0.005 | 98 | Kai | C |
| 2457692.4245 | 2457692.6165 | 15.409 | 0.006 | 213 | Rui | C |
| 2457693.2089 | 2457693.6310 | 15.466 | 0.004 | 551 | Kai | C |
| 2457693.2485 | 2457693.4083 | 15.284 | 0.006 | 208 | Trt | C |
| 2457693.4307 | 2457693.6094 | 1.699 | 0.006 | 228 | Van | C |
| 2457695.4580 | 2457695.5493 | 15.468 | 0.008 | 128 | Trt | C |
| 2457696.2054 | 2457696.5303 | 15.554 | 0.005 | 224 | Trt | C |
| 2457697.2572 | 2457697.3534 | 15.757 | 0.007 | 128 | RPc | V |
| 2457697.2708 | 2457697.3944 | -0.357 | 0.009 | 59 | CRI | C |
| 2457697.9029 | 2457698.1818 | 15.955 | 0.005 | 340 | Ioh | C |
| 2457698.3744 | 2457698.5248 | 15.795 | 0.006 | 200 | RPc | C |
| 2457698.4318 | 2457698.5207 | 15.953 | 0.008 | 105 | Rui | C |
| 2457699.3923 | 2457699.6055 | 15.911 | 0.004 | 233 | RPc | C |
| 2457700.2792 | 2457700.4047 | 15.978 | 0.007 | 131 | RPc | C |
| 2457700.4631 | 2457700.5200 | 16.097 | 0.006 | 70 | deM | C |
| 2457701.2821 | 2457701.4665 | 16.221 | 0.004 | 217 | deM | C |
| 2457702.1912 | 2457702.3770 | 16.118 | 0.006 | 130 | Trt | C |
| 2457702.4545 | 2457702.5813 | 0.809 | 0.006 | 124 | Shu | C |
| 2457702.6942 | 2457702.8284 | 16.415 | 0.002 | 840 | LCO | C |
| 2457702.7029 | 2457702.7335 | 16.186 | 0.019 | 34 | SGE | C |
| 2457703.2716 | 2457703.5612 | 16.595 | 0.005 | 339 | deM | C |
| 2457703.3979 | 2457703.5910 | 16.428 | 0.006 | 135 | RPc | C |
| 2457703.5793 | 2457703.7265 | 16.638 | 0.002 | 663 | LCO | C |
| 2457703.7431 | 2457703.7965 | 16.464 | 0.009 | 76 | SGE | C |
| 2457704.0318 | 2457704.1286 | 3.138 | 0.009 | 261 | KU1 | C |
| 2457705.3068 | 2457705.3939 | 1.251 | 0.164 | 9 | CRI | C |
| 2457705.3462 | 2457705.3527 | 17.825 | 0.069 | 10 | RPc | C |
| 2457710.1836 | 2457710.4889 | 1.172 | 0.007 | 103 | CRI | C |
| 2457711.1870 | 2457711.3958 | 1.441 | 0.008 | 99 | CRI | C |
| 2457712.1411 | 2457712.3578 | 2.867 | 0.008 | 276 | Shu | C |
| 2457712.1620 | 2457712.3942 | 2.251 | 0.018 | 110 | CRI | C |
| 2457713.2081 | 2457713.3496 | 3.784 | 0.020 | 122 | Shu | C |
| 2457714.2452 | 2457714.4152 | 3.788 | 0.018 | 190 | Shu | C |
| 2457715.2334 | 2457715.3837 | 4.121 | 0.019 | 131 | Shu | C |
| 2457718.3214 | 2457718.4191 | 16.762 | 0.004 | 130 | RPc | C |
| 2457721.3110 | 2457721.3110 | 19.486 | – | 1 | RPc | C |
| 2457723.1536 | 2457723.4223 | 4.801 | 0.039 | 97 | Shu | C |
| 2457728.2846 | 2457728.4442 | 5.112 | 0.011 | 151 | Shu | C |

*BJD

†Number of observations.

‡Observer's code and zero-point correction values used in analysis (observations with magnitude larger than 10 reported real magnitudes and others reported differential ones; correction values smaller than −3 and larger than 10 correspond to these two types of observations, respectively): Kai (Kasai, −3.502), Trt (Tordai, −3.326), Rui (Ruiz, −3.497), Van (Vanmunster, 10.296), RPc (Pickard, −3.570), CRI (Crimean Astrophys. Obs., 12.561), Ioh (Itoh, −3.681), deM (de Miguel, −3.529), Shu (Shugarov team, 11.841), LCO (Littlefield, −3.457), SGE (Stone, −3.205), KU (Kyoto U., 10.420)

**E-table 2.** Superhump maxima of OT J002656 during the main superoutburst

| $E$ | max* | error | $O-C$† | $N$‡ | $E$ | max* | error | $O-C$† | $N$‡ |
|---|---|---|---|---|---|---|---|---|---|
| 0 | 57689.2615 | 0.0005 | −0.0087 | 107 | 67 | 57698.1211 | 0.0010 | −0.0081 | 128 |
| 1 | 57689.3953 | 0.0006 | −0.0071 | 94 | 69 | 57698.3822 | 0.0020 | −0.0114 | 78 |
| 2 | 57689.5271 | 0.0005 | −0.0075 | 137 | 70 | 57698.5206 | 0.0006 | −0.0052 | 148 |
| 16 | 57691.3934 | 0.0004 | 0.0077 | 262 | 77 | 57699.4427 | 0.0009 | −0.0087 | 90 |
| 17 | 57691.5254 | 0.0006 | 0.0075 | 147 | 78 | 57699.5747 | 0.0009 | −0.0089 | 114 |
| 23 | 57692.3208 | 0.0005 | 0.0095 | 178 | 84 | 57700.3676 | 0.0011 | −0.0094 | 93 |
| 24 | 57692.4485 | 0.0006 | 0.0049 | 206 | 85 | 57700.5026 | 0.0009 | −0.0066 | 70 |
| 25 | 57692.5834 | 0.0004 | 0.0076 | 101 | 91 | 57701.2929 | 0.0033 | −0.0096 | 75 |
| 30 | 57693.2446 | 0.0006 | 0.0078 | 169 | 92 | 57701.4333 | 0.0012 | −0.0015 | 100 |
| 31 | 57693.3753 | 0.0004 | 0.0062 | 250 | 98 | 57702.2275 | 0.0013 | −0.0006 | 60 |
| 32 | 57693.5083 | 0.0003 | 0.0069 | 279 | 99 | 57702.3603 | 0.0025 | 0.0000 | 52 |
| 33 | 57693.6434 | 0.0020 | 0.0099 | 89 | 100 | 57702.4883 | 0.0009 | −0.0042 | 82 |
| 47 | 57695.4854 | 0.0008 | 0.0007 | 105 | 102 | 57702.7653 | 0.0007 | 0.0083 | 695 |
| 53 | 57696.2761 | 0.0006 | −0.0019 | 75 | 106 | 57703.2885 | 0.0053 | 0.0026 | 78 |
| 54 | 57696.4044 | 0.0010 | −0.0058 | 72 | 107 | 57703.4308 | 0.0016 | 0.0127 | 180 |
| 55 | 57696.5409 | 0.0027 | −0.0016 | 33 | 108 | 57703.5563 | 0.0014 | 0.0059 | 254 |
| 61 | 57697.3290 | 0.0004 | −0.0068 | 160 | 109 | 57703.6937 | 0.0011 | 0.0111 | 423 |
| 66 | 57697.9918 | 0.0010 | −0.0052 | 128 | 112 | 57704.0888 | 0.0026 | 0.0096 | 259 |

*BJD−2400000.

†Against max $= 2457689.2702 + 0.132224E$.

‡Number of points used to determine the maximum.

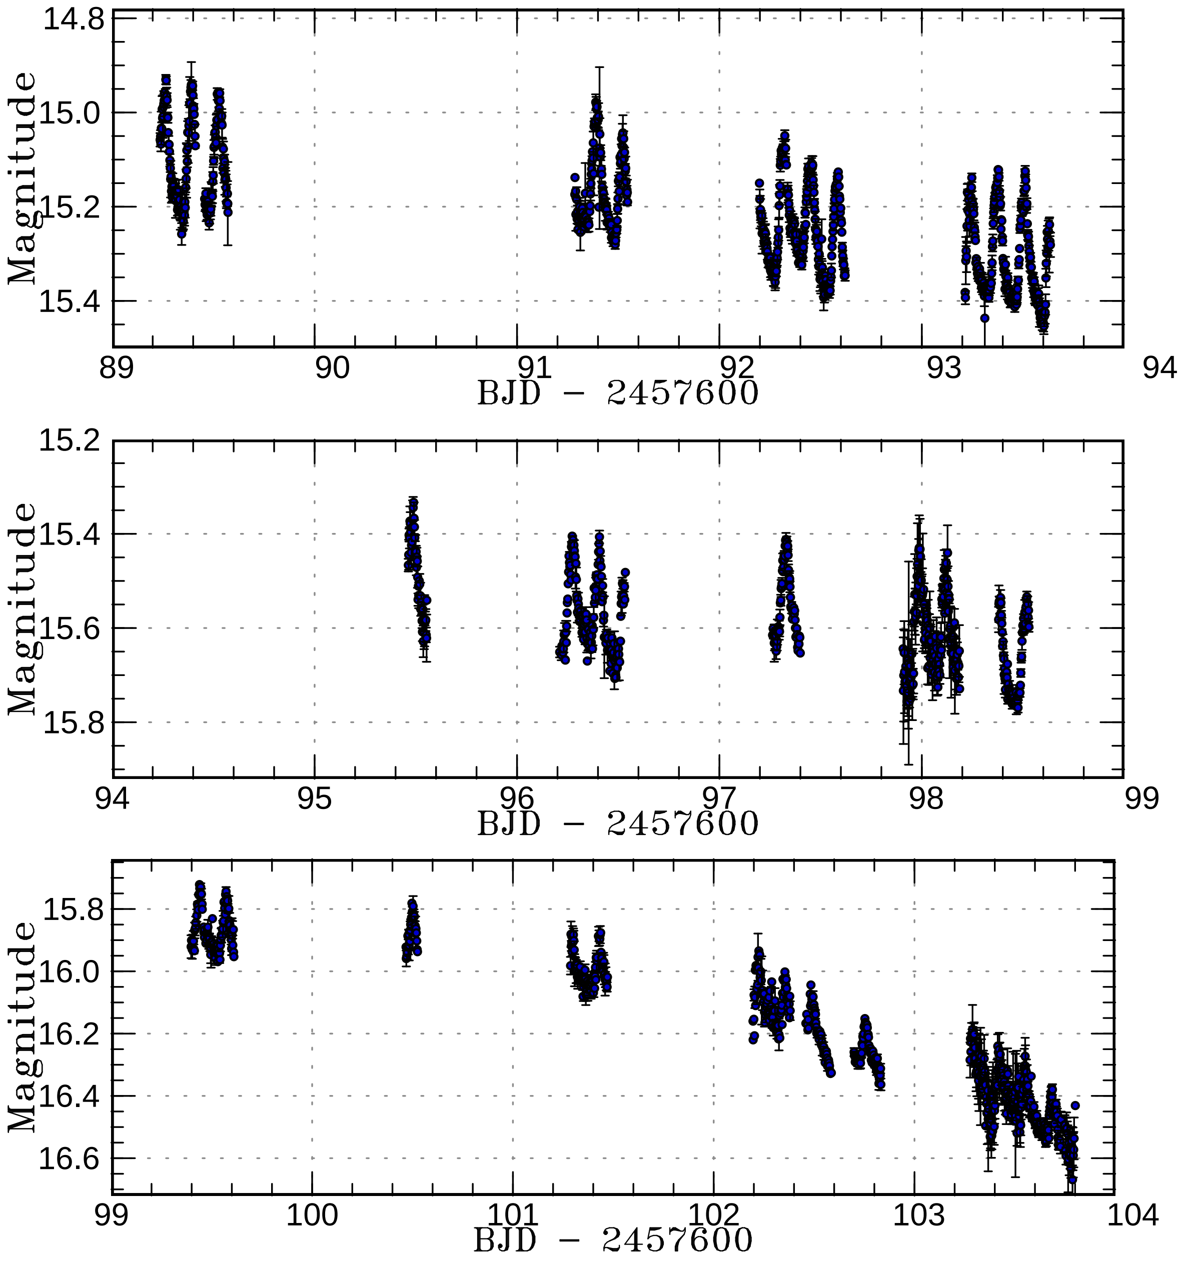


**E-figure 1.** Superhumps in OT J002656 during the superoutburst plateau. The data were binned to 0.002 d.

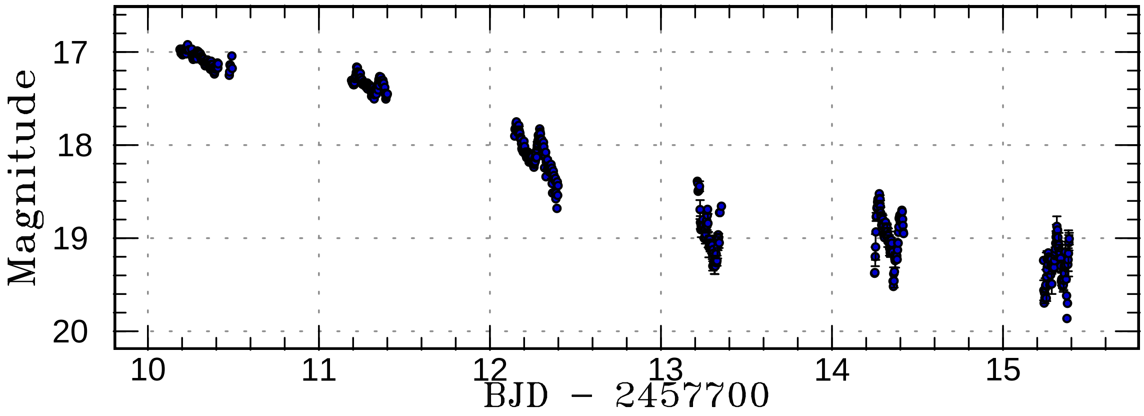


**E-figure 2.** Superhumps in OT J002656 during fading phase of the first rebrightening. The data were binned to 0.002 d.

**E-table 3.** Superhump maxima of OT J002656 after the first re-brightening

| $E$ | max$^*$ | error | $O-C^\dagger$ | $N^\ddagger$ |
|---|---|---|---|---|
| 0 | 57710.3007 | 0.0030 | −0.0057 | 46 |
| 1 | 57710.4452 | 0.0093 | 0.0061 | 15 |
| 7 | 57711.2317 | 0.0014 | −0.0031 | 45 |
| 8 | 57711.3639 | 0.0014 | −0.0035 | 42 |
| 14 | 57712.1730 | 0.0036 | 0.0099 | 139 |
| 15 | 57712.2939 | 0.0018 | −0.0019 | 172 |
| 30 | 57714.2936 | 0.0021 | 0.0085 | 107 |
| 31 | 57714.4073 | 0.0026 | −0.0104 | 78 |

$^*$BJD−2400000.
$^\dagger$Against max $= 2457710.3064 + 0.132620E$.
$^\ddagger$Number of points used to determine the maximum.

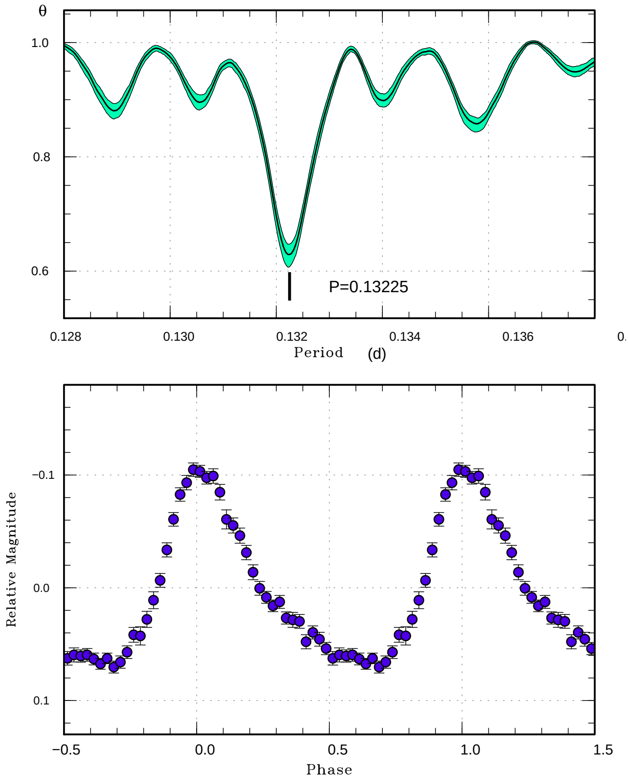


**E-figure 4.** Stage B superhumps in OT J002656. The data between BJD 2457691.6 and 2457705 were used. (Upper): PDM analysis. We analyzed 100 samples which randomly contain 50% of observations, and performed PDM analysis for these samples. The result is shown as a form of 90% confidence intervals in the resultant PDM $\theta$ statistics. (Lower): Phase-averaged profile.

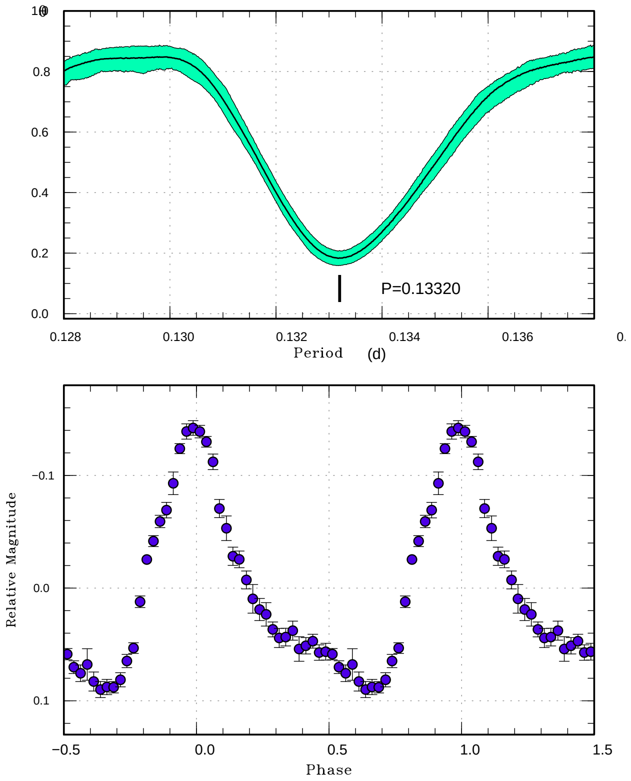


**E-figure 3.** Stage A superhumps in OT J002656. The data before BJD 2457691.6 were used. (Upper): PDM analysis. We analyzed 100 samples which randomly contain 50% of observations, and performed PDM analysis for these samples. The result is shown as a form of 90% confidence intervals in the resultant PDM $\theta$ statistics. (Lower): Phase-averaged profile.

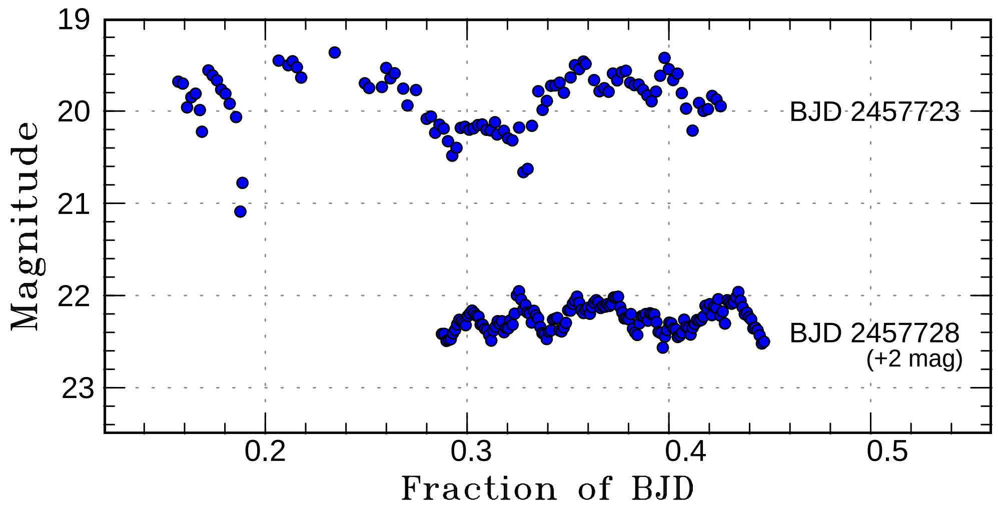


**E-figure 6.** Light curve near quiescence of OT J002656. No clearly periodic signal was detected. The variation was probably dominated by flickering.

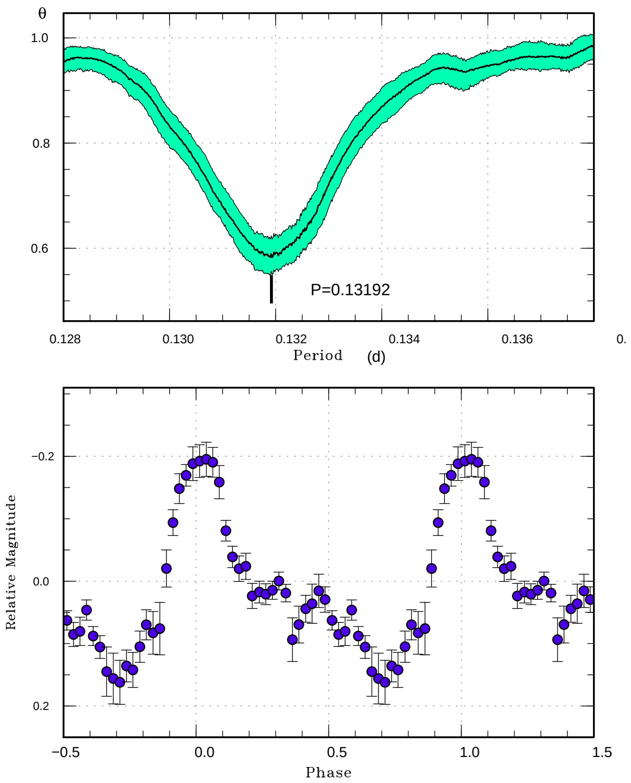


**E-figure 5.** Post-superoutburst superhumps in OT J002656. The data between BJD 2457710 and 2457716 were used. (Upper): PDM analysis. We analyzed 100 samples which randomly contain 50% of observations, and performed PDM analysis for these samples. The result is shown as a form of 90% confidence intervals in the resultant PDM $\theta$ statistics. (Lower): Phase-averaged profile.
